# Supplementary material for: Decays of Majorana or Andreev oscillations induced by steplike spin-orbit coupling
Source: arXiv:1811.06136 source file (2019-04-16)
Supplement: Supplementary file 1 [file decayMBS_Supp_arXiv2.pdf]

# Supplemental Materials
# for
# “Decays of Majorana or Andreev oscillations induced by steplike spin-orbit coupling”

Zhan Cao,[1,2,3,4] Hao Zhang,[5,6] Hai-Feng Lü,[7] Wan-Xiu He,[8] Hai-Zhou Lu,[1,3,4,*] and X. C. Xie[9,6,10]

[1]*Shenzhen Institute for Quantum Science and Engineering and Department of Physics, Southern University of Science and Technology, Shenzhen 518055, China*
[2]*School of Physics, Southeast University, Nanjing 211189, China*
[3]*Peng Cheng Laboratory, Shenzhen 518055, China*
[4]*Shenzhen Key Laboratory of Quantum Science and Engineering, Shenzhen 518055, China*
[5]*State Key Laboratory of Low Dimensional Quantum Physics, Department of Physics, Tsinghua University, Beijing 100084, China*
[6]*Beijing Academy of Quantum Information Sciences, Beijing 100193, China*
[7]*School of Physics, University of Electronic Science and Technology of China, Chengdu 610054, China*
[8]*Center for Interdisciplinary Studies and Key Laboratory for Magnetism and Magnetic Materials of the Ministry of Education, Lanzhou University, Lanzhou 730000, China*
[9]*International Center for Quantum Materials, School of Physics, Peking University, Beijing 100871, China*
[10]*CAS Center for Excellence in Topological Quantum Computation, University of Chinese Academy of Sciences, Beijing 100190, China*

## CONTENTS

SI. Parameters used in Figs. 1(b)-(d) in the main text S1

SII. Effects of magnetic field on the lowest-energy wavefunctions S1

SIII. Origin of decaying or enhanced Majorana oscillations S3

SIV. Effects of tuning various parameters on the Majorana oscillations S4

SV. Origin of decaying Andreev oscillations S5

SVI. An introduction to the measurement of the Majorana oscillations in the semiconductor-superconductor nanowire island S5

References S8

## SI. PARAMETERS USED IN FIGS. 1(B)-(D) IN THE MAIN TEXT

## SII. EFFECTS OF MAGNETIC FIELD ON THE LOWEST-ENERGY WAVEFUNCTIONS

On the top of Fig. 2(a) in the main text, we schematically show that the lowest-energy wavefunctions are squeezed to the interface of the two parts of the nanowire with increasing Zeeman energy $V_Z$. In Fig. S1 we present numerical results to verify this picture. Figs. S1 (a)-(e) and (g)-(k) show the spatial profiles of the wavefunctions $\psi_{e/h}^{L/R}$ corresponding to the lowest-energy spectra $E_{L/R}$ in Figs. 2(b) and (c) in the main text, respectively, at different Zeeman energy. Note that $|\psi_e(x)|^2 = |\psi_h(x)|^2$ due to the particle-hole symmetry of the Hamiltonian studied in the main text. As we can see, the wavefunctions at small Zeeman energies, where the nanowires are in the topologically trivial phase, are extended over the nanowires, while they are localized to the wire ends when the nanowires enter the topological superconducting phase at large enough Zeeman energies. Moreover, as shown in Figs. S1(f) and (l), the wavefunction weights at $x = x_L$ where the entire wire is divided into two parts increase with increasing $V_Z$. As a result, the particle-particle and particle-hole couplings $V_{ee} = \langle\psi_e^L|H|\psi_e^R\rangle$ and $V_{eh} = \langle\psi_e^L|H|\psi_h^R\rangle$, with $H$ the Hamiltonian of the

* Corresponding author: luhaizhou@gmail.com

| | Fig.1(b) | Fig.1(c) | Fig.1(d) | Resonable range |
|---|---|---|---|---|
| $L$ [$\mu$m] | 1.5 | 0.79 | 0.4 | |
| $m^*$ [$m_e$] | 0.046 | 0.072 | 0.125 | 0.026 for bulk InAs [1] |
| $a$ [nm] | 7.5 | 5 | 2.67 | |
| $x_L$ [$\mu$m] | 0.315 | 0.250 | 0.187 | |
| $\Delta$ [meV] | 0.15 | 0.20 | 0.15 | 0.2 for bulk Al [1] |
| $\alpha_0$ [eVÅ] | 0.037 | 0.040 | 0.013 | |
| $A+\alpha_0$ [eVÅ] | 0.187 | 0.294 | 0.398 | 0.2-0.8 for bulk InAs [1] |
| $\mu$ [meV] | 0 | 0.07 | 0.22 | |
| $g_{\text{eff}}$ | 39 | 35 | 33 | 20-50 observed in [2] |

TABLE S1. The parameters used for obtaining the blue solid lines in Figs. 1(b)-(d) in the main text. $a$ is the lattice constant used for simulations. Note that the proximity effects due to the strong tunnel coupling between the namowire and the superconductor not only induce a large effective paring $\Delta$ in the nanowire, but also enhance substantially the effective mass $m^*$ [3]. The parameter renormalization has also been implied in Ref. 4.

entire nanowire (see Sec. *Model* in the main text), are enhanced as $V_Z$ increases, as shown in Fig. 2(e) in the main text.

By diagonalizing the low-energy effective Hamiltonian (Eq. (1) in the main text) one can obtain its eigen-energies

$$\pm E_1 = \pm\left(\sqrt{\varepsilon^2+|V_{eh}|^2}+\sqrt{\delta^2+|V_{ee}|^2}\right), \tag{S1}$$

$$\pm E_2 = \pm\left|\sqrt{\varepsilon^2+|V_{eh}|^2}-\sqrt{\delta^2+|V_{ee}|^2}\right|, \tag{S2}$$

with $\varepsilon=(E_L+E_R)/2$ and $\delta=(E_L-E_R)/2$. The $\pm E_2$ are presented by the blue solid spectrum in Fig. 2(d), which successfully captures the decaying oscillations in the lowest-energy spectrum [Fig. 1(c) in the main text]. The difference between $\pm E_2$ and the exact spectrum is due to neglecting the hybridizations between $E_{L/R}$ and the higher-energy spectrum of the two uncoupled parts of the nanowire.

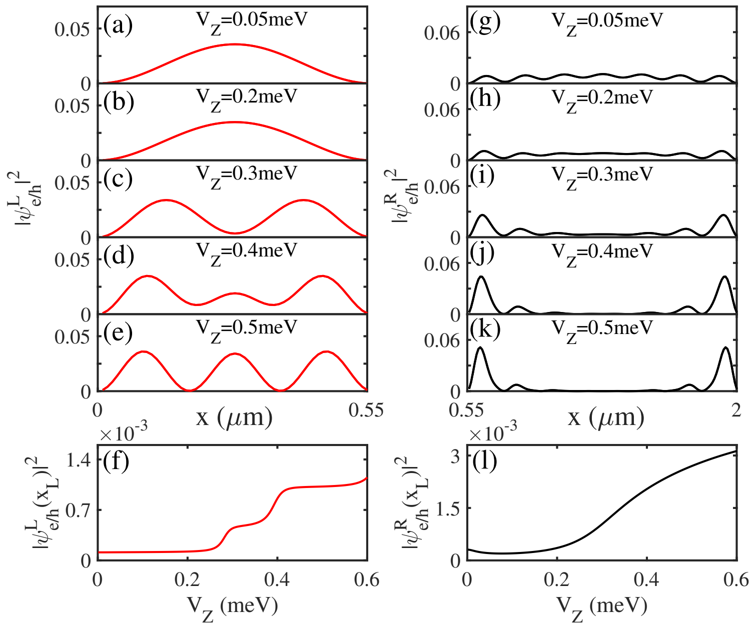


FIG. S1. (Color online) (a)-(e) Spatial profiles of the wavefunctions corresponding to the lowest-energy spectrum in Fig. 2(b) in the main text at different Zeeman energy $V_Z$. (f) The wavefunction weight at $x=x_L=0.55$ $\mu$m, where the entire wire is divided into two parts, is enhanced with increasing $V_Z$. (g)-(l) Similar to (a)-(f) but for the lowest-energy spectrum in Fig. 2(c) in the main text.

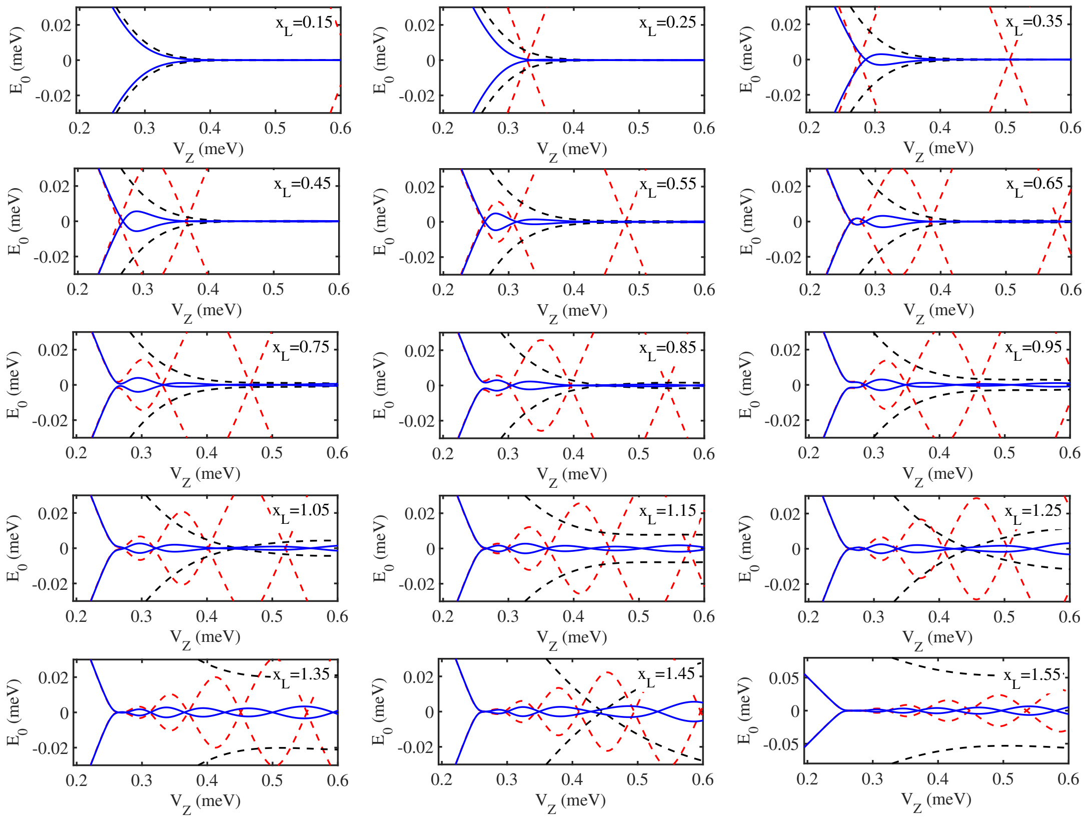


FIG. S2. (Color online) Evolutions of the lowest-energy spectrum when changing $x_L$ from 0.15 $\mu$m to 1.55 $\mu$m with a step 0.1 $\mu$m for a steplike spin-orbit coupling $\alpha(x) = \alpha_0 + A\Theta(x - x_L)$. The blue solid lines represent the exact lowest-energy spectrum of the entire wire, while the red and black dashed lines correspond to the lowest-energy spectra of the left and right parts of the nanowire, which is divided at $x = x_L$. As we explained in the main text, turning on the coupling between the two parts, the red and black dashed spectra hybridize and the repulsion between them repels the lower spectrum towards zero to form the blue solid spectrum. The parameters are the same as those in Fig. 2 in the main text.

## SIII. ORIGIN OF DECAYING OR ENHANCED MAJORANA OSCILLATIONS

In Fig. 2(d) of the main text, we illustrate how the decaying oscillations in the lowest-energy spectrum are formed by the hybridization-induced energy repulsion between the quasi-particle spectra on the two sides of the step. Figure S2 shows the evolutions of the exact lowest-energy spectrum (blue solid line) and $E_{L/R}$ (red and black dashed lines) as we change $x_L$ from 0.15 $\mu$m to 1.55 $\mu$m with a step of 0.1 $\mu$m. The general feature is that the lower energy of the dashed spectra are pushed towards zero to form the blue solid spectrum. Depending on $V_Z$, either the red or black dashed spectrum mainly contributes to the blue solid spectrum. For $x_L > 1.15$, the hybridization-induced energy repulsion is not strong enough to suppress the enhanced oscillations existing in the red dashed spectrum, so the blue solid spectrum of the entire nanowire also shows enhanced oscillations. As shown in the evolutions, at small $x_L$ the first zero-energy crossing in the blue solid spectrum is a crossing. As $x_L$ increases, the crossing turns to alternating crossing and anti-crossing, depending on the red dashed spectrum, as a result of the finite-size effect. The plots for $x_L = 0.35$, 0.55, and 0.75 correspond to the typical patterns observed in the experiments [2, 5–9]. Notably, the oscillation pattern shown in the plot with $x_L = 0.65$ has also been observed in a recent experiment [see Fig. 4(e) of [9]].

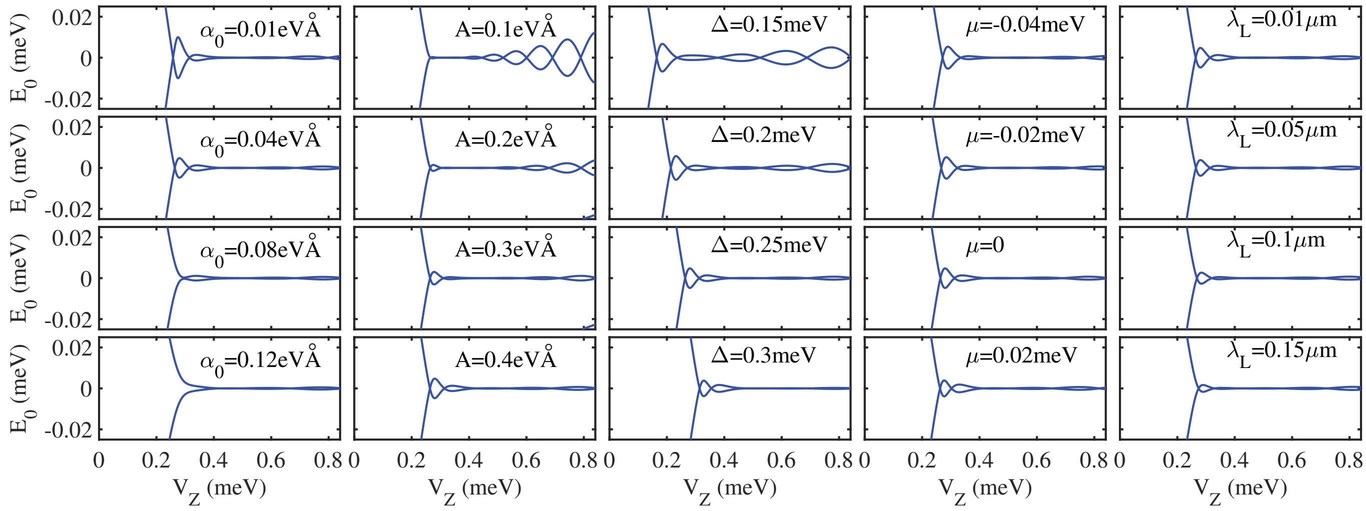


FIG. S3. (Color online) The decaying Majorana oscillations in the lowest-energy spectrum survive when changing various model parameters. Each column shows the evolution of the oscillations when changing one of the model parameters. The parameters except for the one indicated in each subplot are the same as those in Fig. S2.

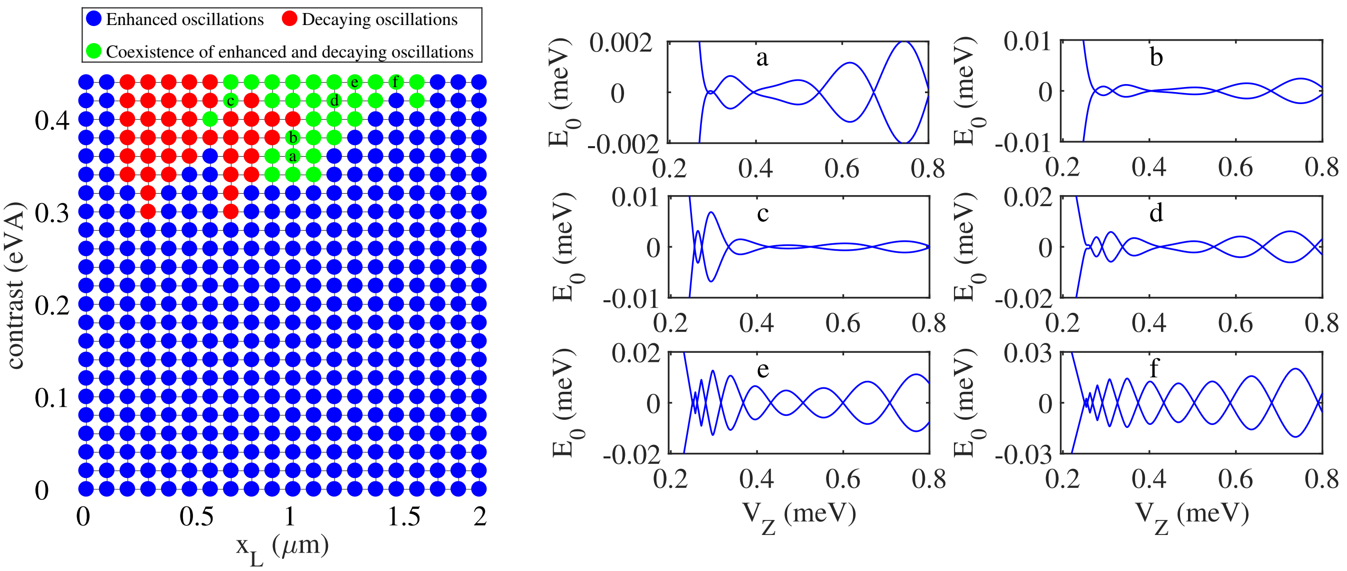


FIG. S4. (Color online) Phase diagram of the oscillation patterns of the lowest-energy spectrum at small magnetic fields. The $x$-axis is $x_L$ and the $y$-axis (contrast) is defined as the difference between the larger spin-orbit coupling (fixed at 0.44 eVÅ) and the smaller spin-orbit coupling on the two sides of the step of the spin-orbit coupling. The oscillation patterns corresponding to the green dots marked by a-f are displayed explicitly in the panels on the right. Upon increasing $x_L$ at a fixed contrast=0.4 eVÅ, detailed evolution of the oscillation patterns is shown in Fig. S2. The parameters are the same as those in Fig. S2.

## SIV. EFFECTS OF TUNING VARIOUS PARAMETERS ON THE MAJORANA OSCILLATIONS

There are several independently adjustable parameters in the Hamiltonian in the main text

$$H = \int_0^L dx \Psi^\dagger(x) \mathcal{H} \Psi(x), \tag{S3}$$

$$\mathcal{H} = \left( \frac{p_x^2}{2m^*} - \mu(x) - \frac{\{\alpha(x), p_x\}}{2\hbar} \sigma_y \right) \tau_z + V_Z \sigma_x + \Delta \tau_x,$$

where $L$, $m^*$, $p_x = -i\hbar\partial_x$, $\Delta$, and $V_Z$ are the wire length, effective electron mass, momentum operator, effective pairing, and Zeeman energy induced by $B$, respectively. $\mu(x)$ and $\alpha(x)$ denote the position-dependent chemical

potential and spin-orbit coupling, respectively. As mentioned in the main text, we employ a steplike spin-orbit coupling $\alpha(x)$

$$\alpha(x) = \frac{A}{2}\left[\tanh\left(\frac{x - x_L}{\lambda_L}\right) + \tanh\left(\frac{x_R - x}{\lambda_R}\right)\right] + \alpha_0, \quad \text{(S4)}$$

where $A$, $\alpha_0$, $x_{L/R}$, and $\lambda_{L/R}$ are the parameters that describe the profile of the steplike spin-orbit coupling.

In Fig. S3, by tuning one of the model parameters while fixing the others, we show that the decaying Majorana oscillations generally survive in the energy spectrum as long as $\alpha_0$ and $A$ have a large enough contrast with a small $\lambda_L$. Moreover, in Fig. S4 we show a phase diagram of the oscillation patterns at small magnetic fields. The $x$-axis is $x_L$ and the $y$-axis (contrast) is defined as the difference between the larger spin-orbit coupling (fixed at 0.44 eVÅ) and the smaller spin-orbit coupling on the two sides of the step of the spin-orbit coupling. The blue, red, and green dots represent the enhanced oscillations, decaying oscillations, and the coexistence of them, respectively. Six oscillation patterns corresponding to the green dots marked by a-f are displayed explicitly in the panels on the right. From this phase diagram, it is clear that the occurrence of decaying oscillations requires both a proper $x_L$ and a large enough contrast.

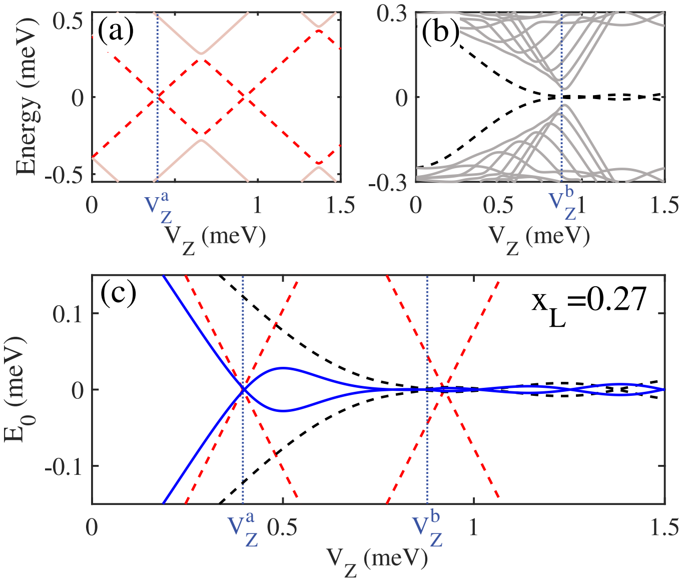


FIG. S5. (Color online) Origin of the decaying Andreev oscillations displayed in Fig. 3(d) in the main text. A 2 $\mu$m nanowire is divided at $x_L = 0.27$ into two parts with different strength of spin-orbit coupling. (a) and (b) show the energy spectra of the left ($\alpha = 0.04$ eVÅ) and right ($\alpha = 0.44$ eVÅ) parts, respectively. (c) Turning on the coupling between the two wires, the lower energy of the dashed spectra are pushed towards zero to form the blue solid spectrum of the entire wire.

## SV. ORIGIN OF DECAYING ANDREEV OSCILLATIONS

Along the same line as the explanation on the decaying Majorana oscillations, we show in Figs. S5 and S6 that the decaying Andreev oscillations displayed in Figs. 3(d) and (e) in the main text are also resulted from the hybridization-induced energy-level repulsion between the red and black dashed energy spectra. In particular, in Figs. S6(d)-(g) we show the spatial profiles of the projections of the lowest-energy wavefunctions of the blue solid spectrum on the Majorana basis at $V_Z$ marked by the scatters in Fig. S6(c). Because the wavefunctions shown in Figs. S6(e) and (f) are separated by a distance comparable with the penetration length, the subgap states in the decaying oscillation regime in Figs. S6(c) are partially separated Andreev bound states [10].

## SVI. AN INTRODUCTION TO THE MEASUREMENT OF THE MAJORANA OSCILLATIONS IN THE SEMICONDUCTOR-SUPERCONDUCTOR NANOWIRE ISLAND

For a better comparison between our theory and the experiments [2, 5–9], we provide a brief introduction to the measurement of the Majorana oscillations in the floating semiconductor-superconductor nanowire island. As shown

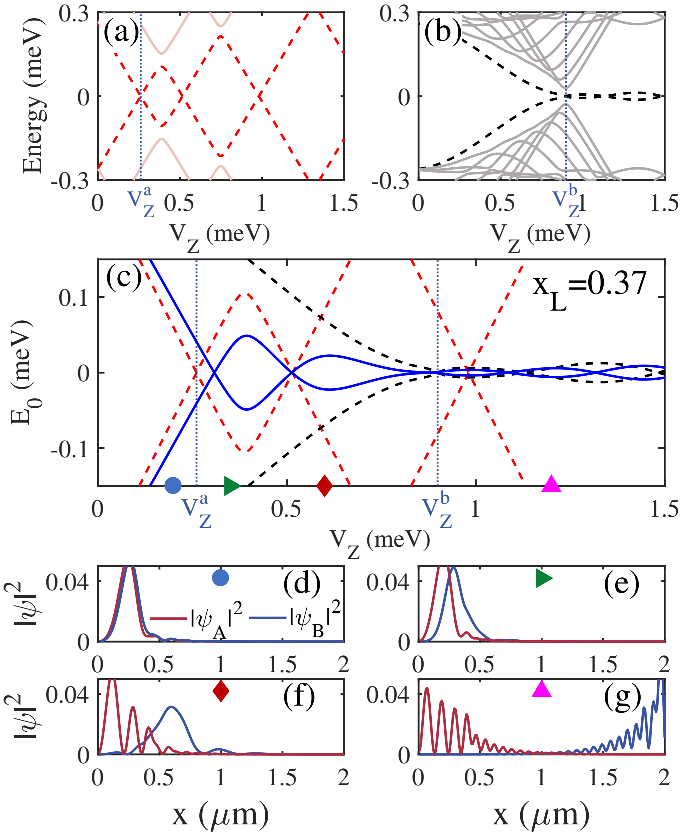


FIG. S6. (Color online) (a)-(c) The same as Fig. S5 for explaining the origin of the decaying Andreev oscillations displayed in Fig. 3(e) in the main text. (d)-(g) Spatial profiles of the projections of the wavefunctions of the lowest-energy states in the blue solid line on the Majorana basis at $V_Z$ marked by the scatters in (c).

in Fig. S7(a), the epitaxially grown superconductor induces an effective pairing $\Delta$ in the nanowire. The bias voltage $V_{\mathrm{SD}}$ drives a charge current $I$ through the island, while the side gate voltages $V_{\mathrm{T1}}$ and $V_{\mathrm{T2}}$ control the tunnel barriers between the metallic leads and their nearby island ends. The plunger gate voltage $V_{\mathrm{G}}$ controls the island electron number by changing the electrostatic energy of the nanowire island

$$E(N) = E_C(N - N_G)^2, \tag{S5}$$

where $N$ is the number of excess electrons, $E_C = e^2/2C$ is the charging energy with $C$ the effective capacitance, and $N_G = CV_G/e$. Above a critical parallel magnetic filed $B$, the island may host the Majorana bound states localized at its two ends. In realistic nanowires within a length of a few micrometers, the hybridization between the Majorana bound states split their energies. The splitting energy $E_0$ has a $B$ dependence, because the wavefunctions of the Majorana bound states depend on the Zeeman energy of the magnetic field. In the weak tunneling regime, the Coulomb blockade effect [11] dominates if $V_{\mathrm{SD}}, k_BT \ll E_C$. Different energy hierarchy of $\Delta$, $E_0$, and $E_C$ determines unique Coulomb blockade patterns [12]. Here, we focus on the relevant regime $E_0 < E_C < \Delta$, where the Majorana oscillations may occur. In this case, the ground-state energy of the nanowire island is

$$E_g(N) = E(N) \tag{S6}$$

if $N$ is an even number (even parity), and

$$E_g(N) = E(N) + E_0 \tag{S7}$$

if $N$ is an odd number (odd parity).

$E_g(N)$ are parabolic functions of $V_G$, with different $N$ corresponding to the bottoms centered at evenly spaced values of $V_G$, as shown in Fig. S7(b). When $V_G$ changes to the values where the neighbouring parabolas cross, e.g., $V_G^{(i)} (i = 1, 2, ...)$ in Fig. S7(b), the ground-state energies with different parities become degenerate, so that an electron

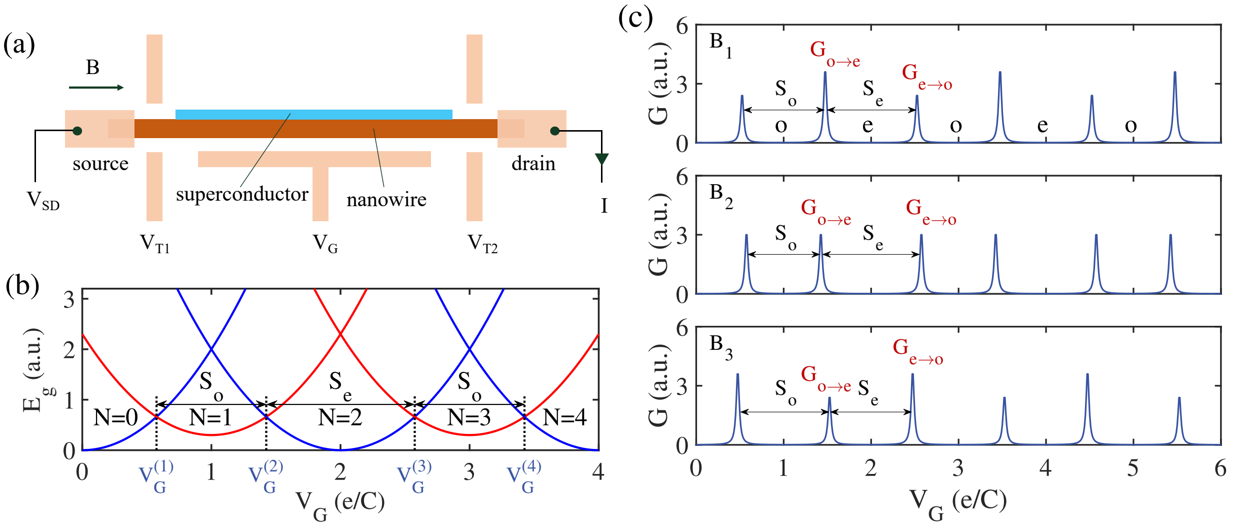


FIG. S7. (Color online) (a) Schematic of charge tunneling experiments through a floating semiconductor-superconductor nanowire island. Applying a parallel magnetic filed $B$ may induce a pair of Majorana bound states at the two ends of the island. The bias voltage $V_{SD}$ drives a charge current $I$ through the island, gate voltages $V_{T1}$, $V_{T2}$ control the tunnel barriers between the metallic leads and their nearest island ends, and $V_G$ controls the island electron number through adjusting the electrostatic energy of the nanowire island [see Eq. (S5)]. (b) Parabolas of the ground-state energy $E_g(N)$ [Eqs. (S6) and (S7)] as a function of the plunger gate voltage $V_G$ with specific electron number $N$ as indicated. The parabolas intersect at $V_G^{(i)}(i = 1, 2, ...)$ and the distances between them are indicated alternatively as $S_o$ and $S_e$, see also (c). (c) Representative experimental Coulomb-blockade peak patterns for three different magnetic fields $B_1$, $B_2$, and $B_3$. Peak spacings for odd (o) and even (e) Coulomb valleys are indicated as $S_o$ and $S_e$, respectively. Peak heights at odd-to-even (even-to-odd) parity transitions occurring upon increasing $V_G$ are denoted as $G_{o\to e}$ ($G_{e\to o}$). Both the peak spacings and peak heights oscillate as $B$ various.

can tunnel into or out of the island without costing an energy, which results in the sharp zero-bias conductance peaks in Fig. S7(c). When $V_G$ deviates from the crossings the island electron number is determined by the state which has the lowest ground-state energy. At zero bias voltage and low temperatures, no energy is available for adding (removing) an electron to (from) the island to the excited state, thus the electron transport through the island is Coulomb blockaded, resulting in the conductance valleys between the conductance peaks in Fig. S7(c). The distances between the crossings of the parabolas are indicated alternatively as $S_o$ and $S_e$ and they are different if $E_0$ is nonzero, as shown below by Eqs. (S11) and (S12). In addition, as schematically shown in Fig. S7(c), upon increasing the gate voltage $V_G$, the conductance peak heights associated to the even-to-odd ($G_{e\to o}$) and odd-to-even ($G_{o\to e}$) ground-state parity transitions are different, due to the fact that they are related to the electron-like and hole-like components of the bound state [13].

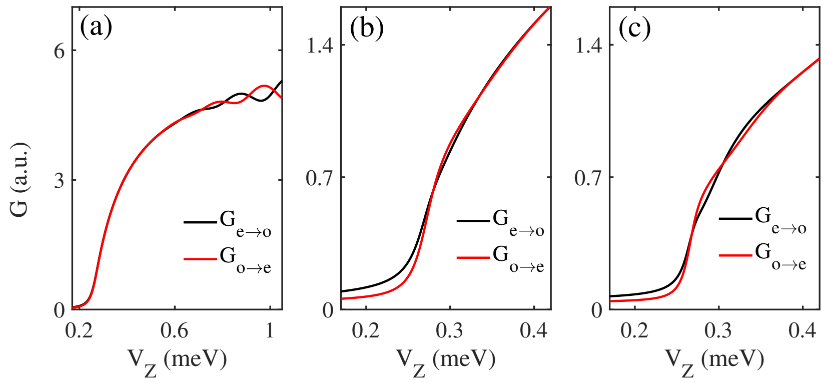


FIG. S8. (Color online) Coulomb-blockade conductance peak heights $G_{e\to o}$ and $G_{o\to e}$ oscillate as functions of the Zeeman energy $V_Z$ for constant (a) and steplike [(b) and (c)] distributions of spin-orbit coupling. The peak height ratio $\Lambda$ shown in Figs. 4(b)-(d) in the main text are obtained by substituting $G_{e\to o}$ and $G_{o\to e}$ shown in (a)-(c) into the definition $\Lambda = G_{e\to o}/(G_{e\to o} + G_{o\to e})$, respectively.

Combining Eqs. (S5)-(S7) one can obtain

$$V_G^{(1)} = \frac{e}{2C}(E_0/E_C + 1), \tag{S8}$$

$$V_G^{(2)} = \frac{e}{2C}(-E_0/E_C + 3), \tag{S9}$$

$$V_G^{(3)} = \frac{e}{2C}(E_0/E_C + 5), \tag{S10}$$

and the peak spacings

$$S_o = V_G^{(2)} - V_G^{(1)} = \eta^{-1}(E_C - E_0), \tag{S11}$$

$$S_e = V_G^{(3)} - V_G^{(2)} = \eta^{-1}(E_C + E_0), \tag{S12}$$

where $\eta = CE_C/e = 2E_C/(S_o + S_e)$. In the experiments [2, 5–9], $E_C$ and $\eta$ were estimated from the Coulomb blockade diamonds and their slopes, respectively. Note that $E_0$ depends on the magnetic filed $B$ as we mentioned above, therefore the peak spacings $S_o$ and $S_o$ varies as $B$ changes, as shown in Fig. S7(c). Eqs. (S11) and (S12) allow one to extract the $E_0$ by the relations $\pm E_0 = \eta\langle S_{e(o)}\rangle - E_C$ with $\langle S_{e(o)}\rangle$ the ensemble-averaged peak spacings, as we mentioned in the caption of Fig. 4 in the main text.

In Figs. 4(b)-(d) in the main text, we show the oscillations of the Coulomb-blockade conductance peak height ratio $\Lambda = G_{e\to o}/(G_{e\to o} + G_{o\to e})$ as a functions of the Zeeman energy for constant and steplike distributions of spin-orbit coupling. In Figs. S8 we plot the corresponding oscillations of $G_{e\to o}$ and $G_{o\to e}$ as functions of the Zeeman energy.


[1] R. Lutchyn, E. Bakkers, L. Kouwenhoven, P. Krogstrup, C. Marcus, and Y. Oreg, "Majorana zero modes in superconductor–semiconductor heterostructures," Nat. Rev. Mater. **3**, 52 (2018).

[2] S. M. Albrecht, A. Higginbotham, M. Madsen, F. Kuemmeth, T. S. Jespersen, J. Nygård, P. Krogstrup, and C. Marcus, "Exponential protection of zero modes in Majorana islands," Nature (London) **531**, 206 (2016).

[3] C. Reeg, D. Loss, and J. Klinovaja, "Metallization of a Rashba wire by a superconducting layer in the strong-proximity regime," Phys. Rev. B **97**, 165425 (2018).

[4] T. D. Stanescu, R. M. Lutchyn, and S. Das Sarma, "Majorana fermions in semiconductor nanowires," Phys. Rev. B **84**, 144522 (2011).

[5] D. Sherman, J. Yodh, S. Albrecht, J. Nygård, P. Krogstrup, and C. Marcus, "Normal, superconducting and topological regimes of hybrid double quantum dots," Nat. Nanotechnol. **12**, 212 (2017).

[6] S. M. Albrecht, E. B. Hansen, A. P. Higginbotham, F. Kuemmeth, T. S. Jespersen, J. Nygård, P. Krogstrup, J. Danon, K. Flensberg, and C. M. Marcus, "Transport signatures of quasiparticle poisoning in a Majorana island," Phys. Rev. Lett. **118**, 137701 (2017).

[7] S. Vaitiekėnas, *et al.*, "Selective-area-grown semiconductor-superconductor hybrids: A basis for topological networks," Phys. Rev. Lett. **121**, 147701 (2018).

[8] E. C. T. O'Farrell, *et al.*, "Hybridization of subgap states in one-dimensional superconductor-semiconductor Coulomb islands," Phys. Rev. Lett. **121**, 256803 (2018).

[9] J. Shen, *et al.*, "Parity transitions in the superconducting ground state of hybrid InSb-Al Coulomb islands," Nat. Commun. **9**, 4801 (2018).

[10] C. Moore, T. D. Stanescu, and S. Tewari, "Two-terminal charge tunneling: Disentangling Majorana zero modes from partially separated Andreev bound states in semiconductor-superconductor heterostructures," Phys. Rev. B **97**, 165302 (2018).

[11] H. Grabert and M. H. Devoret, *Single Charge Tunneling: Coulomb Blockade Phenomena in Nanostructures* (Springer Science & Business Media, New York, 2013), Vol. 294.

[12] B. van Heck, R. M. Lutchyn, and L. I. Glazman, "Conductance of a proximitized nanowire in the Coulomb blockade regime," Phys. Rev. B **93**, 235431 (2016).

[13] E. B. Hansen, J. Danon, and K. Flensberg, "Probing electron-hole components of subgap states in Coulomb blockaded Majorana islands," Phys. Rev. B **97**, 041411(R) (2018).
